# Supplementary material for: Optical modelling of single and multilayer 2D materials and heterostructures
Source: arXiv:2207.11083 ancillary file (2022-11-07)
Supplement: Supplementary file 1 [file supplementary.pdf]

# Optical modelling of 2D materials and multilayer systems: supplementary material

Bruno Majérus and Luc Henrard

*Department of Physics & Namur Institute of Structured Matters (NISM),*

*University of Namur, 61 rue de Bruxelles, B-5000 Namur, Belgium.*

Pascal Kockaert

*OPERA-photonics, Université libre de Bruxelles (U.L.B.),*

*50 Avenue F. D. Roosevelt, CP 194/5, B-1050 Bruxelles, Belgium**

This document is a companion to the article "Optical modelling of 2D materials and multilayer systems: a complete picture". It details long calculation steps. Physical assumptions and interpretations are contained in the main article.

References to equations in the main article are prefixed by "M".

**Contents**

**I. Boundary conditions at the interface** 2

A. Interface matrix from boundary conditions 3

**II. Layer matrix** 4

A. Transmittance and reflectance ratios 5

**III. Interface matrix** 5

A. Interface matrix from layer matrix using backpropagation 6

1. TE configuration 7

2. TM configuration 7

B. Interface matrix from layer matrix in the zero-thickness limit 8

**IV. Volume properties from layer matrix** 8

**V. Poynting vector and transfer matrix** 9

A. Isotropic dielectric surrounding 9

**VI. Upper bound of the error between continuous and discrete models** 11

*Electronic address: Pascal.Kockaert@ulb.ac.be

**VII. Microscopic model versus layer model** 13

A. Microscopic quantities written in the notations of this article 13

B. Comparison with the expressions of the main article 15

## I. BOUNDARY CONDITIONS AT THE INTERFACE

As detailed in [**?** ], boundary conditions for a TE ($\perp$) incident plane wave of frequency $\omega/(2\pi)$, and wavevector $\vec{k} = k_x \vec{1}_x + k_z \vec{1}_x$ on a 2D material located in plane $z = 0$, are (t stands for the transmitted fields, r for the reflected fields, and i for the incident ones)

$$E_y^t = E_y^i + E_y^r, \tag{1}$$

$$k_z^t E_y^t = k_z^i E_y^i + k_z^r E_y^r + \mathrm{i}\mu_0 \omega^2 \mathscr{P}_y, \tag{2}$$

while those for a TM ($\parallel$) wave are

$$D_z^t = D_z^i + D_z^r - \mathrm{i}k_x \mathscr{P}_x, \tag{3}$$

$$\alpha_{it}^{\parallel} D_z^t = D_z^i - D_z^r + \mathrm{i}k_x^2 \frac{\varepsilon_x^i}{k_z^i \varepsilon_0} \mathscr{P}_z, \tag{4}$$

with $\vec{\mathscr{P}}$, the surface polarization field.

For symmetry reasons, it is most of the time possible to assume that the TE and the TM waves are not coupled by the surface polarization term, *i.e.* $\chi_{xz}^s = \chi_{yz}^s = \chi_{zx}^s = \chi_{zy}^s = 0$. In this case, Eqs. (1) and (3); and (2) and (4) write resp.

$$t - r - 1 = \mathrm{i}\varphi_{it}, \tag{5}$$

$$\alpha_{it} t + r - 1 = \mathrm{i}\psi_{it}, \tag{6}$$

with

$$t_\perp = E_y^t / E_y^i, \; r_\perp = E_y^r / E_y^i, \tag{7}$$

$$\alpha_{it}^{\perp} = \frac{k_{z,\perp}^t}{k_{z,\perp}^i}, \; k_{z,TE}^2 = \frac{\varepsilon_x}{\varepsilon_0} k_0^2 - k_x^2, \tag{8}$$

$$\varphi_{it}^{\perp} = 0, \; \psi_{it}^{\perp} = \frac{k_0^2}{k_{z,TE}^i} t_\perp \frac{\mathscr{P}_y}{\varepsilon_0 E_y^t}, \tag{9}$$

$$t_\parallel = D_z^t / D_z^i, \; r_\parallel = D_z^r / D_z^i, \tag{10}$$

$$\alpha_{it}^{\parallel} = \frac{\varepsilon_x^i k_{z,\parallel}^t}{\varepsilon_x^t k_{z,\parallel}^i}, \; k_{z,\parallel}^2 = \frac{\varepsilon_x}{\varepsilon_0} k_0^2 - \frac{\varepsilon_x}{\varepsilon_z} k_x^2, \tag{11}$$

$$\varphi_{it}^{\parallel} = \frac{k_{z,\parallel}^t}{\varepsilon_x^t} t_\parallel \frac{\mathscr{P}_x}{E_x^t}, \; \psi_{it}^{\parallel} = \frac{k_x^2 \varepsilon_x^i}{k_{z,\parallel}^i \varepsilon_0} t_\parallel \frac{\mathscr{P}_z}{D_z^t}, \tag{12}$$

where $k_0^2 = \omega^2 / c^2$, with $c$, the speed of light in a vacuum and $\varepsilon_0$ the permittivity of a vacuum.

### A. Interface matrix from boundary conditions

In [**?** ], it is also shown that the transfer matrix describing the propagation from medium a to medium b (Fig 1 of the main text) should have the form

$$\begin{pmatrix} F_a \\ B_a \end{pmatrix} = \frac{1}{t}\begin{pmatrix} 1 & -r' \\ r & tt' - rr' \end{pmatrix}\begin{pmatrix} F_b \\ B_b \end{pmatrix}, \tag{13}$$

where $r$ and $t$ are the transmission and reflection coefficients appearing in (5) and (6), and their primed version are calculated by swapping indices $a$ and $b$.

We extract $t$ and $r$ from (5) and (6),

$$\frac{1}{t} = \frac{1+\alpha_{ab}}{2} - \mathrm{i}\frac{\varphi_{ab}}{2t} - \mathrm{i}\frac{\psi_{ab}}{2t}, \tag{14}$$

$$\frac{r}{t} = \frac{1-\alpha_{ab}}{2} - \mathrm{i}\frac{\varphi_{ab}}{2t} + \mathrm{i}\frac{\psi_{ab}}{2t}, \tag{15}$$

which allows to calculate $t'$ and $r'$.

This calculation is very long in the general case.

However, if we restrict the calculation to an interface surrounded by vacuum, the expression is simplified and $\alpha_{ab} = 1$ and $\varphi_{ab} = \varphi_{vv} = \varphi_{ba}$, where $v$ denotes the vacuum, and we have also $t = t'$ and $r = r'$. We get

$$\frac{1}{t} = 1 - \mathrm{i}\frac{\varphi_{vv}}{2t} - \mathrm{i}\frac{\psi_{vv}}{2t}, \tag{16}$$

$$\frac{r}{t} = 0 - \mathrm{i}\frac{\varphi_{vv}}{2t} + \mathrm{i}\frac{\psi_{vv}}{2t}, \tag{17}$$

$$-\frac{r'}{t} = 0 + \mathrm{i}\frac{\varphi_{vv}}{2t} - \mathrm{i}\frac{\psi_{vv}}{2t}, \tag{18}$$

$$\frac{tt' - rr'}{t} = t\left[1 - \left(\frac{r}{t}\right)^2\right] \tag{19}$$

$$= \frac{1 - \left(-\mathrm{i}\frac{\varphi_{vv}}{2t} + \mathrm{i}\frac{\psi_{vv}}{2t}\right)^2}{1 - \mathrm{i}\frac{\varphi_{vv}}{2t} - \mathrm{i}\frac{\psi_{vv}}{2t}} \tag{20}$$

$$\overset{\mathcal{O}(1)}{=} 1 + \mathrm{i}\frac{\varphi_{vv}}{2t} + \mathrm{i}\frac{\psi_{vv}}{2t}, \tag{21}$$

and therefore

$$\mathscr{S}_{vv} = \begin{pmatrix} 1 - \mathrm{i}\frac{\varphi_{vv}}{2t} - \mathrm{i}\frac{\psi_{vv}}{2t} & \mathrm{i}\frac{\varphi_{vv}}{2t} - \mathrm{i}\frac{\psi_{vv}}{2t} \\ -\mathrm{i}\frac{\varphi_{vv}}{2t} + \mathrm{i}\frac{\psi_{vv}}{2t} & 1 + \mathrm{i}\frac{\varphi_{vv}}{2t} + \mathrm{i}\frac{\psi_{vv}}{2t} \end{pmatrix}. \tag{22}$$

The general interface matrix between media $a$ and $b$ can be calculated by multiplying standard interface matrices at an interface without surface currents: $\mathscr{I}_{av}$ and $\mathscr{I}_{vb}$. We get

$$\mathscr{S}_{ab} = \mathscr{I}_{av}\mathscr{S}_{vv}\mathscr{I}_{vb}. \tag{23}$$

This is possible only if $\mathscr{S}_{vv}$ is expressed with intrinsic quantities.

Equations (9) and (12) have the right form for this, as $E_x$, $E_y$ and $D_z$ are continuous accross the boundary. This is a direct consequence of (1), (3) and (4) for an interface without surface currents ($\vec{\mathscr{P}} = \vec{0}$) which means that we can decompose any interface matrix according to $\mathscr{I}_{ab} = \mathscr{I}_{av}\mathscr{I}_{vb}$, and assume that these three components are the same in $a$, $v$ and $b$.

## II. LAYER MATRIX

The matrix of a layer of material $m$ surrounded by vacuum is calculated using

$$\begin{aligned}
&\mathscr{L}_m(d) \\
&= \mathscr{I}_{vm}\mathscr{P}_m(d)\mathscr{I}_{mv} && (24)\\
&= \begin{pmatrix} \frac{1+\alpha}{2} & \frac{1-\alpha}{2} \\ \frac{1-\alpha}{2} & \frac{1+\alpha}{2} \end{pmatrix} \begin{pmatrix} e^{-i\Phi} & 0 \\ 0 & e^{i\Phi} \end{pmatrix} \begin{pmatrix} \frac{\alpha+1}{2\alpha} & \frac{\alpha-1}{2\alpha} \\ \frac{\alpha-1}{2\alpha} & \frac{\alpha+1}{2\alpha} \end{pmatrix} && (25)\\
&= \begin{pmatrix} \cos\Phi - i\frac{1+\alpha^2}{2\alpha}\sin\Phi & i\frac{1-\alpha^2}{2\alpha}\sin\Phi \\ -i\frac{1-\alpha^2}{2\alpha}\sin\Phi & \cos\Phi + i\frac{1+\alpha^2}{2\alpha}\sin\Phi \end{pmatrix}, && (26)
\end{aligned}$$

where $\alpha = \alpha_{vm} = 1/\alpha_{mv}$, $\Phi = k_z^m d$, and $\alpha_{mn}$ and $k_z^m$ are defined in I.

As the phase shift $\Phi$ is very small, we can write

$$\exp(i\Phi) = \frac{\exp(i\Phi/2)}{\exp(-i\Phi/2)} = \frac{\cos(\Phi/2) + i\sin(\Phi/2)}{\cos(\Phi/2) - i\sin(\Phi/2)} = \frac{1 + i\tan(\Phi/2)}{1 - i\tan(\Phi/2)}, \tag{27}$$

so that

$$\begin{aligned}
\exp(i\Phi) &= \frac{1 + i\Phi/2 + \mathscr{O}\left(\Phi^3\right)}{1 - i\Phi/2 + \mathscr{O}\left(\Phi^3\right)}, && (28)\\
2\cos\Phi &= \exp(i\Phi) + \exp(-i\Phi) && (29)\\
&\overset{\mathscr{O}(2)}{=} \frac{1 + i\Phi/2}{1 - i\Phi/2} + \frac{1 - i\Phi/2}{1 + i\Phi/2} = \frac{(1 + i\Phi/2)^2 + (1 - i\Phi/2)^2}{(1 + i\Phi/2)(1 - i\Phi/2)} && (30)\\
&= 2\frac{1 - \Phi^2/4}{1 + \Phi^2/4}, && (31)\\
2i\sin\Phi &= \exp(i\Phi) - \exp(-i\Phi) && (32)\\
&\overset{\mathscr{O}(2)}{=} \frac{1 + i\Phi/2}{1 - i\Phi/2} - \frac{1 - i\Phi/2}{1 + i\Phi/2} = \frac{(1 + i\Phi/2)^2 - (1 - i\Phi/2)^2}{(1 + i\Phi/2)(1 - i\Phi/2)} && (33)\\
&= 2i\frac{2\Phi/2}{1 + \Phi^2/4}. && (34)
\end{aligned}$$

Using these relations in (26), we get the conservative approximation of the transfer matrix of a layer

$$\begin{pmatrix} \frac{4-\Phi^2}{4+\Phi^2} - i\frac{1+\alpha^2}{\alpha}\frac{2\Phi}{4+\Phi^2} & i\frac{1-\alpha^2}{\alpha}\frac{2\Phi}{4+\Phi^2} \\ -i\frac{1-\alpha^2}{\alpha}\frac{2\Phi}{4+\Phi^2} & \frac{4-\Phi^2}{4+\Phi^2} + i\frac{1+\alpha^2}{\alpha}\frac{2\Phi}{4+\Phi^2} \end{pmatrix}. \tag{35}$$

### A. Transmittance and reflectance ratios

From (35), we extract

$$\begin{aligned}
T_L &= \frac{\alpha_{vm}\left(4+\Phi_m^2\right)}{\alpha_{vm}\left(4-\Phi_m^2\right)-\mathrm{i}2\Phi_m\left(1+\alpha_{vm}^2\right)} && (36)\\
&= \frac{\alpha_{vm}\left(4+\Phi_m^2\right)}{\left(2\alpha_{vm}-\mathrm{i}\Phi_m\right)\left(2-\mathrm{i}\alpha_{vm}\Phi_m\right)} && (37)\\
&= \frac{1}{2}\frac{\left(2+\mathrm{i}\Phi_m/\alpha_{vm}\right)\left(2-\mathrm{i}\alpha_{vm}\Phi_m\right)+\left(2-\mathrm{i}\Phi_m/\alpha_{vm}\right)\left(2+\mathrm{i}\alpha_{vm}\Phi_m\right)}{\left(2-\mathrm{i}\Phi_m/\alpha_{vm}\right)\left(2-\mathrm{i}\alpha_{vm}\Phi_m\right)} && (38)\\
&= \frac{1}{2}\left(\frac{2+\mathrm{i}\Phi_m/\alpha_{vm}}{2-\mathrm{i}\Phi_m/\alpha_{vm}}+\frac{2+\mathrm{i}\alpha_{vm}\Phi_m}{2-\mathrm{i}\alpha_{vm}\Phi_m}\right) && (39)\\
&= \frac{1}{2}\left[\frac{\left(2-\mathrm{i}\Phi_m/\alpha_{vm}\right)+2\mathrm{i}\Phi_m/\alpha_{vm}}{2-\mathrm{i}\Phi_m/\alpha_{vm}}+\frac{\left(2-\mathrm{i}\alpha_{vm}\Phi_m\right)+2\mathrm{i}\alpha_{vm}\Phi_m}{2-\mathrm{i}\alpha_{vm}\Phi_m}\right] && (40)\\
&= 1+\frac{\mathrm{i}\Phi_m/\alpha_{vm}}{2-\mathrm{i}\Phi_m/\alpha_{vm}}+\frac{\mathrm{i}\alpha_{vm}\Phi_m}{2-\mathrm{i}\alpha_{vm}\Phi_m} && (41)\\
R_L &= \frac{-\mathrm{i}2\Phi_m\left(1-\alpha_{vm}^2\right)}{\left(2\alpha_{vm}-\mathrm{i}\Phi_m\right)\left(2-\mathrm{i}\alpha_{vm}\Phi_m\right)} && (42)\\
&= \frac{2}{2-\mathrm{i}\alpha_{vm}\Phi_m}-\frac{2}{2-\mathrm{i}\Phi_m/\alpha_{vm}} && (43)\\
&= \frac{\mathrm{i}\alpha_{vm}\Phi_m}{2-\mathrm{i}\alpha_{vm}\Phi_m}-\frac{\mathrm{i}\Phi_m/\alpha_{vm}}{2-\mathrm{i}\Phi_m/\alpha_{vm}}. && (44)
\end{aligned}$$

To compare these expressions to the boundary conditions (5) and (6), we write

$$\begin{aligned}
T_L-R_L &= 1+\frac{2\mathrm{i}\Phi_m/\alpha_{vm}}{2-\mathrm{i}\Phi_m/\alpha_{vm}}, && (45)\\
T_L+R_L &= 1+\frac{2\mathrm{i}\alpha_{vm}\Phi_m}{2-\mathrm{i}\alpha_{vm}\Phi_m}, && (46)
\end{aligned}$$

and so

$$\begin{aligned}
T_L\left(\frac{1}{T_L}+\frac{R_L}{T_L}-1\right) &= -\frac{2\mathrm{i}\Phi_m/\alpha_{vm}}{2-\mathrm{i}\Phi_m/\alpha_{vm}}, && (47)\\
T_L\left(\frac{1}{T_L}-\frac{R_L}{T_L}-1\right) &= -\frac{2\mathrm{i}\alpha_{vm}\Phi_m}{2-\mathrm{i}\alpha_{vm}\Phi_m}. && (48)
\end{aligned}$$

The layer matrix cannot be directly related to the boundary conditions, as the layer matrix has a thickness, and the interface not.

## III. INTERFACE MATRIX

We can obtain the interface matrix from the layer matrix in two different ways, based on the assumption that the current sheet is located in the middle of the layer and surrounded by vacuum.

### A. Interface matrix from layer matrix using backpropagation

In a first approach, we remove the thickness of the layer matrix by propagating over a negative distance on both sides:

$$\mathscr{S}_{vv}^{m} = \mathscr{P}_v(-d/2)\mathscr{L}_m(d)\mathscr{P}_v(-d/2). \tag{49}$$

This results in transmission $T_S$ and reflexion $R_S$ coefficients for the current sheet

$$\frac{T_S}{T_L} = \mathrm{e}^{-\mathrm{i}\Phi_v}, \tag{50}$$

$$\frac{R_S}{R_L} = \mathrm{e}^{-\mathrm{i}\Phi_v}. \tag{51}$$

To expand these expressions, we define $\rho_\pm = T_L(1/T_L \pm R_L/T_L - 1)$, and $\mathrm{i}\kappa_\pm = \frac{-2\rho_\pm}{2-\rho_\pm}$ so that

$$\rho_+ = -\frac{2\mathrm{i}\Phi_m/\alpha_{vm}}{2-\mathrm{i}\Phi_m/\alpha_{vm}} = -\frac{2\mathrm{i}\kappa_+}{2-\mathrm{i}\kappa_+}, \tag{52}$$

$$\rho_- = -\frac{2\mathrm{i}\Phi_m\alpha_{vm}}{2-\mathrm{i}\Phi_m\alpha_{vm}} = -\frac{2\mathrm{i}\kappa_-}{2-\mathrm{i}\kappa_-}, \tag{53}$$

$$\kappa_+ = \Phi_m/\alpha_{vm}, \tag{54}$$

$$\kappa_- = \Phi_m\alpha_{vm} \tag{55}$$

and

$$T_S\left(\frac{1}{T_S} \pm \frac{R_S}{T_S} - 1\right) = 1 + \mathrm{e}^{-\mathrm{i}\Phi_v} T_L\left(\pm\frac{R_L}{T_L} - 1\right) \tag{56}$$

$$= 1 + \mathrm{e}^{-\mathrm{i}\Phi_v}\left(\rho_\pm - 1\right) \tag{57}$$

$$\approx 1 + \frac{2-\mathrm{i}\Phi_v}{2+\mathrm{i}\Phi_v}\left(\frac{-2\mathrm{i}\kappa_\pm}{2-\mathrm{i}\kappa_\pm} - 1\right) \tag{58}$$

$$= 1 + \frac{2-\mathrm{i}\Phi_v}{2+\mathrm{i}\Phi_v}\left(-\frac{2+\mathrm{i}\kappa_\pm}{2-\mathrm{i}\kappa_\pm}\right) \tag{59}$$

$$\approx 1 - \frac{4+2(\mathrm{i}\kappa_\pm - \mathrm{i}\Phi_v)}{4-2(\mathrm{i}\kappa_\pm - \mathrm{i}\Phi_v)} = -\frac{2\mathrm{i}(\kappa_\pm - \Phi_v)}{2-\mathrm{i}(\kappa_\pm - \Phi_v)}, \tag{60}$$

where we have neglected terms on the order of $\kappa\Phi_v$. The last expression is similar to $\rho_\pm$ provided that we replace $\kappa_\pm$ with $\kappa_\pm - \Phi_v$. We can therefore write

$$T_S\left(\frac{1}{T_S} + \frac{R_S}{T_S} - 1\right) = -\frac{2\mathrm{i}(\Phi_m/\alpha_{vm} - \Phi_v)}{2-\mathrm{i}(\Phi_m/\alpha_{vm} - \Phi_v)}, \tag{61}$$

$$T_S\left(\frac{1}{T_S} - \frac{R_S}{T_S} - 1\right) = -\frac{2\mathrm{i}(\Phi_m\alpha_{vm} - \Phi_v)}{2-\mathrm{i}(\Phi_m\alpha_{vm} - \Phi_v)}. \tag{62}$$

To find explicit expressions, we must consider separately the definitions of $\alpha$ and $\Phi$ for TE and TM modes.

### 1. TE configuration

In this configuration, we get

$$\alpha_{vm}\Phi_m - \Phi_v = \frac{\left(k_z^m\right)^2}{k_z^v} d_m - k_z^v d_m = \frac{d_m}{k_z^v}\left(\left(k_z^m\right)^2 - \left(k_z^v\right)^2\right) \tag{63}$$

$$= \frac{d_m}{k_z^v}\left(\varepsilon_y^m k_0^2 - k_0^2\right) = \frac{k_0^2}{k_z^v} d_m \left(\frac{\varepsilon_y^m}{\varepsilon_0} - 1\right) = \frac{k_0^2}{k_z^v}\left[\chi_y^m d_m\right], \tag{64}$$

$$\Phi_m/\alpha_{vm} - \Phi_v = \frac{k_z^v}{k_z^m} k_z^m d_m - k_z d_m = 0, \tag{65}$$

and making the parallel between (5)-(6) and (61)-(62), at first order, we get

$$\varphi^\perp = \frac{k_0^2}{k_z^v}\left[\chi_y^m d_m\right] = \frac{k_0^2}{k_z^v}\chi_y^{s,m}, \tag{66}$$

$$\psi^\perp = 0, \tag{67}$$

in which we have defined the surface susceptibility as $\chi^s = d\chi$.

### 2. TM configuration

In this configuration, we get

$$\alpha_{vm}\Phi_m - \Phi_m = \varepsilon_0 \frac{\left(k_z^m\right)^2}{\varepsilon_x^m k_z} d_m - k_z^v d_m \tag{68}$$

$$= \varepsilon_0 \frac{d_m}{k_z^v}\left(k_0^2 - \frac{k_x^2}{\varepsilon_z^m}\right) - \varepsilon_0 \frac{d_m}{k_z^v}\left(k_0^2 - k_x^2\right) \tag{69}$$

$$= \frac{d_m}{k_z^v} k_x^2 \left(1 - \frac{1}{\varepsilon_z^m}\right) = \frac{k_x^2}{k_z^v}\left[\frac{\varepsilon_z^m - 1}{\varepsilon_z^m} d_m\right] \tag{70}$$

$$= \frac{k_x^2}{k_z^v}\left[\xi_z^m d_m\right], \tag{71}$$

$$\Phi_m/\alpha_{vm} - \Phi_m = \frac{\varepsilon_x^m k_z^v}{\varepsilon_0 k_z^m} k_z^m d_m - k_z^v d_m = k_z^v \left[\left(\frac{\varepsilon_x^m}{\varepsilon_0} - 1\right) d_m\right] \tag{72}$$

$$= k_z^v \left[\chi_x^m d_m\right] \tag{73}$$

where we have defined the displacement permittivity $\xi_z^m = \frac{\varepsilon_z^m - 1}{\varepsilon_z^m}$.

Making the parallel between (5)-(6) and (61)-(62), at first order, we get

$$\varphi^\parallel = \frac{k_x^2}{k_z^v}\left[\xi_z^m d_m\right] = \frac{k_x^2}{k_z^v}\xi_z^{s,m}, \tag{74}$$

$$\psi^\parallel = k_z^v \left[\chi_x^m d_m\right] = k_z^v \chi_x^{s,m}, \tag{75}$$

in which we have defined the surface quantities $\chi^s = d\chi$ and $\xi^s = d\xi$.

### B. Interface matrix from layer matrix in the zero-thickness limit

Equations (64), (71) and (73) can be written as

$$[\alpha_{vm}\Phi_m]_\perp = \Phi_m + \frac{k_x^2}{k_z^v}\xi_z^{m,s}, \tag{76}$$

$$= k_z^v d_m + \frac{k_0^2}{k_z^v}\chi_y^{m,s}, \tag{77}$$

$$[\alpha_{vm}\Phi_m]_\parallel = k_z^v d_m + \frac{k_x^2}{k_z^v}\xi_z^{m,s}, \tag{78}$$

$$[\Phi_m/\alpha_{vm}]_\parallel = k_z^v d_m + k_z^v \chi_x^{m,s}, \tag{79}$$

with the previous definitions of the surface quantities: $q^s = dq$, $q = \chi, \xi$. This shows that the surface quantities can be identified by taking the limit

$$\lim_{d_m \to 0} \rho_\pm, \tag{80}$$

in the TE and TM configuration. This provides another way to consider the surface quantities as

$$\chi_x^s = \lim_{d_m\to 0}\left[d_m\left(\frac{\varepsilon_x-\varepsilon_0}{\varepsilon_0}\right)\right] = \lim_{d_m\to 0}\left[d_m\varepsilon_x\right]/\varepsilon_0, \tag{81}$$

$$\chi_y^s = \lim_{d_m\to 0}\left[d_m\left(\frac{\varepsilon_y-\varepsilon_0}{\varepsilon_0}\right)\right] = \lim_{d_m\to 0}\left[d_m\varepsilon_y\right]/\varepsilon_0, \tag{82}$$

$$\xi_z^s = \lim_{d_m\to 0}\left[d_m\left(\frac{\varepsilon_z-\varepsilon_0}{\varepsilon_z}\right)\right] = \lim_{d_m\to 0}\left[-\frac{d_m}{\varepsilon_z}\right]\varepsilon_0. \tag{83}$$

## IV. VOLUME PROPERTIES FROM LAYER MATRIX

The differential equation

$$\frac{\mathrm{d}\mathcal{V}_m}{\mathrm{d}D} = K_m\mathcal{V}_m, \tag{84}$$

with

$$K_m = \mathrm{i}k_z^m \mathcal{I}_{vm}\begin{pmatrix} -1 & 0 \\ 0 & 1 \end{pmatrix}\mathcal{I}_{mv}, \tag{85}$$

admits for solution the matrix exponential

$$\mathcal{V}_m = \mathrm{e}^{K_m D} I = \mathrm{e}^{\mathrm{i}k_z^m D \mathcal{I}_{vm}\begin{pmatrix} -1 & 0 \\ 0 & 1 \end{pmatrix}\mathcal{I}_{mv}}. \tag{86}$$

To provide an explicit form for this exponential, it is necessary to work in a basis where the matrix $K_m$ is diagonal.

To this end, we rewrite the differential equation after a change of variables $U = \mathscr{I}_{mv}\mathscr{V}_m$,

$$\frac{\mathrm{d}U_m}{\mathrm{d}D} = \mathscr{I}_{mv}\, K_m\, \mathscr{I}_{vm}\, U_m = \mathrm{i}k_z^m \begin{pmatrix} -1 & 0 \\ 0 & 1 \end{pmatrix} U_m, \tag{87}$$

leading to

$$U_m(D) = \mathrm{e}^{\mathrm{i}k_z^m D \begin{pmatrix} -1 & 0 \\ 0 & 1 \end{pmatrix}} U_m(0) = \begin{pmatrix} \mathrm{e}^{-\mathrm{i}k_z^m D} & 0 \\ 0 & \mathrm{e}^{\mathrm{i}k_z^m D} \end{pmatrix} U_m(0), \tag{88}$$

$$\mathscr{V}_m = \mathscr{I}_{vm} U = \mathscr{I}_{vm} \begin{pmatrix} \mathrm{e}^{-\mathrm{i}k_z^m D} & 0 \\ 0 & \mathrm{e}^{\mathrm{i}k_z^m D} \end{pmatrix} \mathscr{I}_{mv}, \tag{89}$$

where the solution $\mathscr{V}_m(0) = I$ was used. This provides $U_m(0) = \mathscr{I}_{mv}$.

## V. POYNTING VECTOR AND TRANSFER MATRIX

The conservation of the energy flux is based on the Poynting verctor $\vec{S}$. To avoid considering the surface on which the flux is integrated, it is easier to integrate the flux on the interface surface, which is equivalent to consider only the normal component to the interface $S_z$.

This component writes in TE and TM configurations

$$S_z^\perp = \gamma^2 \mathrm{Re}\left[k_z^\perp\right] |E_y^2| \tag{90}$$

$$= \gamma^2 \mathrm{Re}\left[k_z^\perp\right] |F_\perp|^2, \tag{91}$$

$$S_z^\parallel = \gamma^2 k_0^2 \mathrm{Re}\left[\frac{\varepsilon_x}{k_z^\parallel}\right] |E_x^2| \tag{92}$$

$$= \gamma^2 k_0^2 \mathrm{Re}\left[\frac{k_z^\parallel}{\varepsilon_x}\right] \left|\frac{\varepsilon_x}{k_z^\parallel}\right|^2 |E_x^2| \tag{93}$$

$$= \gamma^2 k_0^2 \mathrm{Re}\left[k_z^\parallel/\varepsilon_x\right] |F_\parallel|^2, \tag{94}$$

where $\gamma$ is a normalization factor, and $F_\perp$ and $F_\parallel$ are the quantities used to evaluate $r$ and $t$ [see (7) and (10)].

### A. Isotropic dielectric surrounding

If the material is lossless and surrounded by a lossless isotropic material, there are no losses and the flux should be conserved

$$S_z^i = S_z^r + S_z^t, \tag{95}$$

which leads to

$$1 = |r|^2 + \alpha_{ti}|t|^2, \tag{96}$$

or

$$\frac{1}{|t|^2} - \frac{|r|^2}{|t|^2} = \alpha_{ti}, \tag{97}$$

For the layer and the interface model, we have

$$R_L = \frac{\mathrm{i}\kappa_+}{2-\mathrm{i}\kappa_+} - \frac{\mathrm{i}\kappa_-}{2-\mathrm{i}\kappa_-} = -\frac{\rho_+}{2} + \frac{\rho_-}{2} \tag{98}$$

$$T_L = 1 + \frac{\mathrm{i}\kappa_+}{2-\mathrm{i}\kappa_+} + \frac{\mathrm{i}\kappa_-}{2-\mathrm{i}\kappa_-} = 1 - \frac{\rho_+}{2} - \frac{\rho_-}{2} \tag{99}$$

$$\alpha_{ti} = \alpha_{mm} = 1, \tag{100}$$

$$R_S = R_L|_{\kappa_\pm \to \kappa_\pm - \Phi_v} \tag{101}$$

$$T_S = T_L|_{\kappa_\pm \to \kappa_\pm - \Phi_v} \tag{102}$$

To verify the conservation of the flux, we calculate

$$|T_L|^2 = 1 + \frac{|\rho_+|^2}{4} + \frac{|\rho_-|^2}{4} - \mathrm{Re}[\rho_+] - \mathrm{Re}[\rho_-] + \frac{\mathrm{Re}[\rho_+\rho_-^*]}{2} \tag{103}$$

$$|R_L|^2 = \frac{|\rho_+|^2}{4} + \frac{|\rho_-|^2}{4} - \frac{\mathrm{Re}[\rho_+\rho_-^*]}{2} \tag{104}$$

$$|T_L|^2 + |R_L|^2 = 1 + \frac{|\rho_+|^2}{2} + \frac{|\rho_-|^2}{2} - \mathrm{Re}[\rho_+] - \mathrm{Re}[\rho_-] \tag{105}$$

Now, we calculate $|\rho|^2$ and $\mathrm{Re}[\rho]$ under the assumption that $\kappa$ is real. We get

$$|\rho|^2 = \frac{4\kappa^2}{4+\kappa^2}, \tag{106}$$

$$\mathrm{Re}[\rho] = \mathrm{Re}\left[-\frac{2\mathrm{i}\kappa}{2-\mathrm{i}\kappa}\right] = \mathrm{Re}\left[-\frac{2\mathrm{i}\kappa(2+\mathrm{i}\kappa)}{4+\kappa^2}\right] = 2\frac{\kappa^2}{4+\kappa^2} \tag{107}$$

$$= \frac{|\rho|^2}{2}, \tag{108}$$

$$\frac{|\rho|^2}{2} - \mathrm{Re}[\rho] = 0. \tag{109}$$

This shows that $|T_L|^2 + |R_L|^2 = 1$, as requested by flux conservation.

We could perform the same calculation with $R_S$ and $T_S$ and would get the same result, provided that $k_z$ is real.

## VI. UPPER BOUND OF THE ERROR BETWEEN CONTINUOUS AND DISCRETE MODELS

Here, we provide an upper bound for the phase difference $\Delta\Phi$ between the discrete and the continuous layer models

$$\Delta\Phi = \Phi_c - \Phi_d = \Phi_c - \ln(1 + \mathrm{i}\Phi_c)/\mathrm{i}. \tag{110}$$

We start by separating real and imaginary parts

$$\mathrm{i}\Phi_c = -\alpha + \mathrm{i}\theta, \tag{111}$$

$$\mathrm{i}\Phi_c - \mathrm{i}\Phi_d = -\alpha + \mathrm{i}\theta - \ln(1-\alpha+\mathrm{i}\theta) \tag{112}$$

$$= -\alpha + \mathrm{i}\theta - \ln\left[\sqrt{(1-\alpha)^2+\theta^2}\,\mathrm{e}^{\mathrm{i}\tan^{-1}\frac{\theta}{1-\alpha}}\right] \tag{113}$$

$$= -\alpha + \mathrm{i}\theta - \frac{1}{2}\ln\left[(1-\alpha)^2+\theta^2\right] - \mathrm{i}\tan^{-1}\frac{\theta}{1-\alpha}. \tag{114}$$

We will now find an upper bound separately for

$$R(\alpha,\theta) = -\alpha - \frac{1}{2}\ln\left[(1-\alpha)^2+\theta^2\right], \tag{115}$$

$$I(\alpha,\theta) = \theta - \tan^{-1}\frac{\theta}{1-\alpha}. \tag{116}$$

A classical and efficient manner to find the upper bound is to develop the function in Taylor series and use the Taylor integral remainder. As $R$ and $I$ depend on two variables, we introduce ancilary functions $\tilde{R}(t)$ and $\tilde{I}(t)$ defined by

$$\tilde{R}(t) = R(t\alpha, t\theta), \tag{117}$$

$$\tilde{I}(t) = I(t\alpha, t\theta), \tag{118}$$

so that, for each of the two functions $R$ and $I$, we have

$$F(\alpha,\theta) = \tilde{F}(1) = \tilde{F}(0) + \int_0^1 \tilde{F}'\mathrm{d}t = \tilde{F}(0) + 1\cdot\tilde{F}'(0) + \int_0^1 \frac{(1-t)^1}{1!}\tilde{F}''|_t\mathrm{d}t. \tag{119}$$

*a. Real term* We get successively

$$\tilde{R}(t) = -t\alpha - \frac{1}{2}\ln(1-t\alpha)^2 - \frac{1}{2}\ln\left[1+\frac{t^2\theta^2}{(1-t\alpha)^2}\right] \tag{120}$$

$$= -\left[t\alpha + \ln(1-t\alpha)\right] - \frac{1}{2}\ln\left[1+\frac{t^2\theta^2}{(1-t\alpha)^2}\right] \tag{121}$$

$$= \tilde{R}_1 + \tilde{R}_2, \tag{122}$$

$$\tilde{R}_1'(t) = -\left[\alpha - \alpha\frac{1}{1-t\alpha}\right] = \frac{t\alpha}{1-t\alpha}, \tag{123}$$

$$\tilde{R}_2'(t) = -\frac{1}{2}\left(\frac{2t\theta^2}{(1-t\alpha)^2} + 2\alpha\frac{t^2\theta^2}{(1-t\alpha)^3}\right)\frac{1}{1+\frac{t^2\theta^2}{(1-t\alpha)^2}} \tag{124}$$

$$= -\frac{t\theta^2}{(1-t\alpha)^3}\left(\frac{1}{1+\frac{t^2\theta^2}{(1-t\alpha)^2}}\right) \tag{125}$$

$$\tilde{R}_1''(t) = \frac{\alpha^2}{(1-t\alpha)^2} \tag{126}$$

$$\tilde{R}_1(1) = 0+0+\int_0^1 (1-t)\frac{\alpha^2}{(1-t\alpha)^2}\mathrm{d}t \tag{127}$$

$$\leq \frac{\alpha^2}{(1-\alpha)^2}\int_0^1 (1-t)\mathrm{d}t \leq \frac{\alpha^2}{2(1-\alpha)^2}, \tag{128}$$

$$-\tilde{R}_2(1) = 0+\int_0^1 \frac{t\theta^2}{(1-t\alpha)^3}\left(\frac{1}{1+\frac{t^2\theta^2}{(1-t\alpha)^2}}\right)\mathrm{d}t \tag{129}$$

$$\leq \frac{1}{(1-\alpha)^3}\int_0^1 t\theta^2\mathrm{d}t = \frac{\theta^2}{2(1-\alpha)^3}, \tag{130}$$

$$|R(\alpha,\theta)| \leq \frac{\alpha^2+\theta^2}{2(1-\alpha)^3} = \frac{|\varphi|^2}{2(1-\alpha)^3}, \tag{131}$$

where we make the assumption that $0 \leq \alpha < 1$.

*b. Imaginary term* We get

$$\tilde{I}(t) = t\theta - \tan^{-1}\frac{t\theta}{1-t\alpha} = t\theta - \tan^{-1}\frac{\theta}{\frac{1}{t}-\alpha}, \tag{132}$$

$$\tilde{I}'(t) = \theta - \frac{\theta}{(1-t\alpha)^2}\left(\frac{1}{1+\left(\frac{\theta}{1/t-\alpha}\right)^2}\right), \tag{133}$$

$$\tilde{I}''(t) = -2\alpha\frac{\theta}{(1-t\alpha)^3}\frac{1}{\left[1+\left(\frac{\theta}{1/t-\alpha}\right)^2\right]} - 2\frac{1}{t^2}\frac{\theta^2}{(1/t-\alpha)^2}\frac{1}{\left[1+\left(\frac{\theta}{1/t-\alpha}\right)^2\right]^2}, \tag{134}$$

$$I(\alpha,\beta) = 0+0+\int_0^1 (1-t)\tilde{I}''(t)\mathrm{d}t, \tag{135}$$

$$\left|I(\alpha,\beta)\right| \leq \sqrt{\frac{\alpha^2\theta^2}{(1-\alpha)^6}+\frac{\theta^4}{(1-\alpha)^4}} \leq \sqrt{\frac{\alpha^2\theta^2}{(1-\alpha)^6}+\frac{\theta^4}{(1-\alpha)^6}} = \frac{|\theta\varphi|}{(1-\alpha)^3} \leq \frac{|\varphi|^2}{(1-\alpha)^3}. \tag{136}$$

*c. Global upper bound*

$$|R(\alpha,\theta)| \leq \frac{|\varphi|^2}{2(1-\alpha)^3}, \tag{137}$$

$$\left|I(\alpha,\beta)\right| \leq \frac{|\theta\varphi|}{(1-\alpha)^3}, \tag{138}$$

$$\sqrt{R^2+I^2} \leq \frac{|\varphi|}{(1-\alpha)^3}\sqrt{\alpha^2/2+3\theta^2/2} \leq \frac{3}{2}\frac{|\varphi|^2}{(1-\alpha)^3}, \tag{139}$$

$$|\Delta\Phi| = |\Phi_c - \Phi_d| \leq \frac{3}{2}\frac{|\Phi_c|^2}{(1-\mathrm{Im}\,[\Phi_c])^3} \tag{140}$$

which is a global upper bound. The error on the attenuation and the phase can also be evaluated separately

$$|\alpha_c - \alpha_d| \leq \frac{|\varphi_c|^2}{2(1-\alpha_c)^3}, \tag{141}$$

$$|\theta_c - \theta_d| \leq \frac{|\theta_c \varphi_c|}{(1-\alpha_c)^3} \leq \frac{|\varphi_c|^2}{(1-\alpha_c)^3}. \tag{142}$$

## VII. MICROSCOPIC MODEL VERSUS LAYER MODEL

### A. Microscopic quantities written in the notations of this article

In [**?** , Eq. 4], the reflection coefficient is given as

$$r_{sp} = -\frac{n\cos\theta - \cos\theta_t}{n\cos\theta + \cos\theta_t} + R_\parallel + R_\perp, \tag{143}$$

$$R_\parallel = \frac{n\cos\theta - \cos\theta_t + (\mathrm{i}k\chi_\parallel + \sigma_\parallel\eta)\cos\theta\cos\theta_t}{n\cos\theta + \cos\theta_t + (\mathrm{i}k\chi_\parallel + \sigma_\parallel\eta)\cos\theta\cos\theta_t}, \tag{144}$$

$$R_\perp = \frac{n^2\cos\theta - n\cos\theta_t - (\mathrm{i}k\chi_\perp + \sigma_\perp\eta)\sin^2\theta}{n^2\cos\theta + n\cos\theta_t + (\mathrm{i}k\chi_\perp + \sigma_\perp\eta)\sin^2\theta}. \tag{145}$$

We first introduce the complex permittivity $\chi_i$, so that

$$(\mathrm{i}k\chi_\perp + \sigma_\perp\eta) = \mathrm{i}k_0\chi_z, \tag{146}$$

$$(\mathrm{i}k\chi_\parallel + \sigma_\parallel\eta) = \mathrm{i}k_0\chi_x. \tag{147}$$

Moreover, taking into account that $n_i = 1$, and $n_t = n$ the trigonometric functions of the input and transmitted angles can be replaced as follows

$$\sin\theta = \frac{k_x}{k_0}, \tag{148}$$

$$\cos\theta = \frac{k_z^i}{k_0}, \tag{149}$$

$$\cos\theta_t = \frac{k_z^t}{k_0 n}, \tag{150}$$

so that

$$r_{sp} = -\frac{k_z^i - k_z^t/n^2}{k_z^i + k_z^t/n^2} + R_\parallel + R_\perp, \tag{151}$$

$$R_\parallel = \frac{k_z^i - k_z^t/n^2 + \mathrm{i}\chi_x k_z^i k_z^t/n^2}{k_z^i + k_z^t/n^2 + \mathrm{i}\chi_x k_z^i k_z^t/n^2}, \tag{152}$$

$$R_\perp = \frac{k_z^i - k_z^t/n^2 - \mathrm{i}\chi_z k_x^2/n^2}{k_z^i + k_z^t/n^2 + \mathrm{i}\chi_z k_x^2/n^2}. \tag{153}$$

Now, we introduce $\alpha_{it}$ and $n^2 = \varepsilon_x^t$ as in this configuration $n_i = 1$ and $n_t = n$, so that

$$k_z^t/n^2 = \alpha_{it} k_z^i, \tag{154}$$

to get

$$\begin{aligned} r_{sp} &= -\frac{1-\alpha_{it}}{1+\alpha_{it}} + \frac{1-\alpha_{it}+\mathrm{i}\chi_x k_z^t/n_t^2}{1+\alpha_{it}+\mathrm{i}\chi_x k_z^t/n_t^2} \\ &\quad + \frac{1-\alpha_{it}-\mathrm{i}\left(\chi_z/n_t^2\right)k_x^2/k_z^i}{1+\alpha_{it}+\mathrm{i}\left(\chi_z/n_t^2\right)k_x^2/k_z^i}. \end{aligned} \tag{155}$$

Applying the same succession of operations, we can turn the reflectivity for the immersed 2D material as follows

$$r_{ip} = R_\parallel + R_\perp, \tag{156}$$

$$R_\parallel = \frac{\left(\mathrm{i}k\chi_\parallel + \sigma_\parallel \eta\right)\cos\theta}{2n + \left(\mathrm{i}k\chi_\parallel + \sigma_\parallel\eta\right)\cos\theta} \tag{157}$$

$$= \frac{\mathrm{i}k_0\chi_x \cos\theta/n}{2+\mathrm{i}k_0\chi_x\cos\theta/n} \tag{158}$$

$$= \frac{\mathrm{i}k_z^a\chi_x/n^2}{2+\mathrm{i}k_z^a\chi_x/n^2} = \frac{\mathrm{i}\tau_x}{2+\mathrm{i}\tau_x}, \tag{159}$$

$$\tau_x = k_z^a\chi_x/n^2, \tag{160}$$

$$R_\perp = \frac{-n\left(\mathrm{i}k\chi_\perp + \sigma_\perp\eta\right)\sin^2\theta}{2\cos\theta + n\left(\mathrm{i}k\chi_\perp+\sigma_\perp\eta\right)\sin^2\theta} \tag{161}$$

$$= \frac{-\mathrm{i}k_0\chi_z n^2 \sin^2\theta}{2n\cos\theta + \mathrm{i}k_0\chi_z n^2\sin^2\theta}, \tag{162}$$

$$= \frac{-\mathrm{i}\frac{k_x^2}{k_z^a}\chi_z}{2+\mathrm{i}\frac{k_x^2}{k_z^a}\chi_z} = \frac{-\mathrm{i}\tau_z}{2+\mathrm{i}\tau_z}, \tag{163}$$

$$\tau_z = \frac{k_x^2}{k_z^a}\chi_z, \tag{164}$$

and similarly, using for the TE configuration the coefficients provided in [**?** ], and $\alpha_{it} = \frac{k_z^t}{k_z^i}$

$$r_{ss} = \frac{n_i\cos\theta - n_t\cos\theta_t - \left(\mathrm{i}k\chi + \sigma\eta\right)}{n_i\cos\theta + n_t\cos\theta_t + \left(\mathrm{i}k\chi+\sigma\eta\right)} \tag{165}$$

$$= \frac{k_z^i - k_z^t - \mathrm{i}k_0^2\chi_y}{k_z^i + k_z^t + \mathrm{i}k_0^2\chi_y} \tag{166}$$

$$= \frac{1-\alpha_{it} - \mathrm{i}\frac{k_0^2}{k_z^i}\chi_y}{1+\alpha_{it}+\mathrm{i}\frac{k_0^2}{k_z^i}\chi_y}. \tag{167}$$

For the immersed layer, where $n_t = n_i = n_a$ and $\alpha_{it} = 1$, we get

$$r_{is} = \frac{-\mathrm{i}\frac{k_0^2}{k_z^a}\chi_y}{2+\mathrm{i}\frac{k_0^2}{k_z^a}\chi_y} = \frac{-\mathrm{i}\tau_y}{2-\tau_y}, \tag{168}$$

$$\tau_y = \frac{k_0^2}{k_z^a}\chi_y. \tag{169}$$

### B. Comparison with the expressions of the main article

The immersed configuration can be obtained from the layer model as follows, with $a$ indicating parameters of the polymer layer

$$\begin{aligned}\mathcal{M}^m_{aa} &= \mathcal{I}_{av}\mathcal{L}_m(d_m)\mathcal{I}_{va} = \mathcal{I}_{av}\mathcal{I}_{vm}\mathcal{P}_m(d_m)\mathcal{I}_{mv}\mathcal{I}_{va} \\ &= \mathcal{I}_{am}\mathcal{P}_m(d_m)\mathcal{I}_{ma}. \end{aligned} \tag{170}$$

As the coefficient $\alpha$ in (M11) comes from the interface matrix and $\Phi_m$ comes from the propagation matrix, it is sufficient to replace $\alpha_{vm}$ by $\alpha_{am}$ in (M31) and (M32) to find the expression for an immersed layer of material $m$. To go from this thick layer to the interface model, we can then let $d_m \to 0$ as described in Sec. M4, and detailed in III.

Writing

$$\kappa_x = \lim_{d_m\to 0} \Phi_m^{\parallel}/\alpha_{am}^{\parallel} = \frac{k_z^a\varepsilon_0}{\varepsilon_x^a}\chi_x^s, \tag{171}$$

$$\kappa_y = \lim_{d_m\to 0} \Phi_m^{\perp}\alpha_{am}^{\perp} = \frac{k_0^2}{k_z^a}\chi_y^s, \tag{172}$$

$$\kappa_z = \lim_{d_m\to 0} \Phi_m^{\parallel}\alpha_{am}^{\parallel} = \frac{k_x^2\varepsilon_x^a}{k_z^a\varepsilon_0}\xi_z^s, \tag{173}$$

$$\tag{174}$$

(M31) provides the reflection coefficients

$$R_S^{\perp} = \frac{\mathrm{i}\kappa_y}{2-\mathrm{i}\kappa_y}, \tag{175}$$

$$R_S^{\parallel} = -\frac{\mathrm{i}\kappa_x}{2-\mathrm{i}\kappa_x} + \frac{\mathrm{i}\kappa_z}{2-\mathrm{i}\kappa_z}, \tag{176}$$

for a 2D material immersed in medium $a$.

A comparison of (M31) and (M32) with (159)–(163) shows that these expressions are identical if $\kappa_i = \tau_i$, $i = x, y, z$. This occurs when

$$\chi_z^s = n_a^2\xi_z^s. \tag{177}$$

and we take the same sign convention for the Fourier transform.
